# Supplementary material for: Benchmark on Peer Review Toxic Detection: A Challenging Task with a New Dataset
Source: arXiv:2502.01676 source file (2025-02-01)
Supplement: Supplementary file 1 [file appendix.tex]

\section{Detoxify Generation Evaluation Prompts}
To automatically evaluate if a detoxified sentence is indeed better than an original toxic sentence, or how a base model revision compares to a fine-tuned revision, we prompt GPT-4 to evaluate. The following is the prompt that we use.

\begin{lstlisting}[linewidth=\columnwidth,breaklines=true,breakautoindent=false,breakindent=0pt]
The following are two sentences from scientific paper reviews:

1. {sentence1}
2. {sentence2}

Choose the sentence that is more conducive to a productive and encouraging review environment by answering either '1' or '2'. 
\end{lstlisting}
    % \caption{Our prompt for judging between two sentences with GPT-4.}
\label{fig:prompt}
The sentence order is randomized to avoid order bias. \\

We also utilized GPT-4 to judge the quality of a revision more similarly to our human review using the following prompt.

\begin{lstlisting}[linewidth=\columnwidth,breaklines=true,breakautoindent=false,breakindent=0pt]
The following is a sentence from a scientific paper review:

" {sentence} "

Here is a revised version of that same sentence:

" {revision} "

If this revision a) conveys the content of the original sentence faithfully, b) improves the tone such that it is more encouraging and/or constructive, AND c) makes sense in the context of a paper review environment, then it qualifies as a good revision. All criteria must be met for a revision to qualify.

Does this qualify? Answer with YES or NO.
\end{lstlisting}
    % \caption{Our prompt for evaluating revision quality with GPT-4.}
\label{fig:prompt}

\section{More Experiments Results}

Here, we also provide the performance of toxic classification task on each label. 
\begin{table}[t]
\centering
 \resizebox{0.98\linewidth}{!}{
\begin{tabular}{c|c|c|c}
    \toprule
    \multirow{2}{*}{\textbf{Models}}& \multicolumn{3}{c}{\textbf{Performance}}\\
     \cmidrule(lr){2-4}
     & {\textbf{Precision}} &  {\textbf{Recall}}  & {\textbf{F1}} \\ 
     \toprule
    ChatGPT 3.5 Zero-shot& 0.766& 0.606& 0.677\\
    Mistral 7B Zero-shot& 0.814& 0.802& 0.701\\
    Zephyr  3B Zero-shot& 0.445& 0.902& 0.596\\
    Llama 3 Zero-shot& 0.678& 0.913& 0.778\\
    Our method (Fine-tuned Mistral)& 0.814& 0.802& 0.808\\
    Our method (Fine-tuned Zephyr)& 0.798& 0.793& 0.795\\
    Our method (DeBerta-v3+Random Forest)& 0.876& 0.815& 0.844\\
    \bottomrule
    \end{tabular}
    }
    \vspace{3mm}
\caption{Toxic label performance.}
\label{tab:detector_result_toxic_2}
\end{table}

\begin{table}[t]
\centering
 \resizebox{0.98\linewidth}{!}{
\begin{tabular}{c|c|c|c}
    \toprule
    \multirow{2}{*}{\textbf{Models}}& \multicolumn{3}{c}{\textbf{Performance}}\\
     \cmidrule(lr){2-4}
     & {\textbf{Precision}} &  {\textbf{Recall}}  & {\textbf{F1}} \\ 
     \toprule
    ChatGPT 3.5 Zero-shot& 0.871& 0.935& 0.902\\
    Mistral 7B Zero-shot& 0.909& 0.857& 0.883\\
    Zephyr  3B Zero-shot& 0.946& 0.602& 0.736\\
    Llama 3 Zero-shot& 0.965& 0.847& 0.902\\
    Our method (Fine-tuned Mistral)& 0.931& 0.935& 0.933\\
    Our method (Fine-tuned Zephyr)& 0.927& 0.929& 0.928\\
    Our method (DeBerta-v3+Random Forest)& 0.786& 0.854& 0.818\\
    \bottomrule
    \end{tabular}
    }
    \vspace{3mm}
\caption{Non-Toxic label performance.}
\label{tab:detector_result_toxic_3}
\end{table}
